# Supplementary material for: Plasmons on the edge of MoS2 nanostructures
Source: arXiv:1503.00538 source file (2015-03-02)
Supplement: Supplementary file 1 [file supplemental.pdf]

# Supplementary Material for Plasmons on the Edge of $MoS_2$ Nanostructures

Kirsten Andersen,[1,*] Karsten W. Jacobsen,[1] and Kristian S. Thygesen[1,2]

[1] *Center for Atomic-scale Materials Design, Department of Physics*
*Technical University of Denmark, DK - 2800 Kgs. Lyngby, Denmark*
[2] *Center for Nanostructured Graphene*
*Technical University of Denmark, DK - 2800 Kgs. Lyngby, Denmark*

## I. STRUCTURE OF THE $MoS_2$ RIBBON

The structure of the ribbon used for the calculations is shown in Fig. 1.

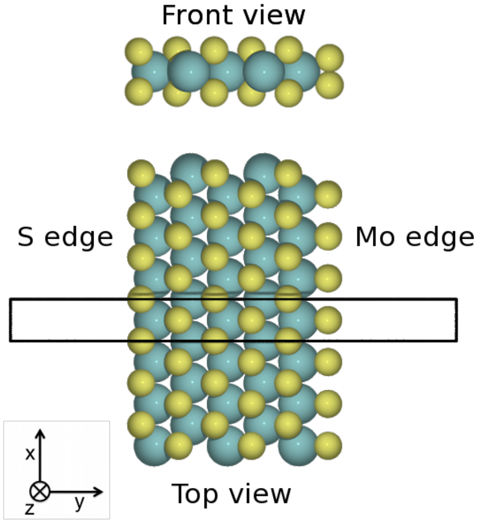


FIG. 1: Front and top-view of the $MoS_2$ ribbon used for the DFT calculations. The Mo- and S-edge, covered by S-dimers, is found to the left and right respectively. The width of the ribbon is approximately 1.5 nm, and the supercell includes 20 and 12 Å of vacuum in the $y$ and $z$ direction respectively. The black black insert shows the unit cell that is repeated in the calculation.

## II. SPATIALLY RESOLVED EELS

The loss spectrum is defined as the power dissipated in the medium due to an external potential, $\phi_{ext}(\mathbf{r})e^{i\omega t}$:

$$P(\omega) = \int\int d\mathbf{r}d\mathbf{r}'\phi_{ext}(\mathbf{r})\chi(\mathbf{r},\mathbf{r}',\omega)\phi_{ext}(\mathbf{r}'). \quad (1)$$

Here $\chi$ is the interacting density response function. In the case of EELS, the external potential corresponds to the Coulomb potential of a fast electron moving at constant velocity $\mathbf{v}_e$ emitted at point $\mathbf{r}_0$:

$$\phi_{ext}(\mathbf{r},t) = \frac{4\pi e^2}{|\mathbf{r}-\mathbf{r}_0-\mathbf{v}_e t|}, \quad (2)$$

which in Fourier space takes the form:

$$\phi_{ext}(\mathbf{q},\omega) = \int dt \frac{1}{\mathbf{q}^2} e^{-i\mathbf{q}\cdot\mathbf{r}_0} e^{i(\omega-\mathbf{q}\cdot\mathbf{v}_e)t} = \frac{1}{\mathbf{q}^2} e^{-i\mathbf{q}\cdot\mathbf{r}_0}\delta(\omega-\mathbf{q}\cdot\mathbf{v}_e). \quad (3)$$

---

* kiran@fysik.dtu.dk

This leads to the expression for the power dissipation:

$$P(\omega) = \sum_{\mathbf{q}_x} \sum_{\mathbf{G},\mathbf{G}'} \frac{e^{i(\mathbf{G}+\mathbf{q}_x)\cdot\mathbf{r}_0}}{|\mathbf{q}_x + \mathbf{G}|^2} \chi_{\mathbf{G},\mathbf{G}'}(\mathbf{q}_x,\omega) \frac{e^{-i(\mathbf{G}'+\mathbf{q}_x)\cdot\mathbf{r}_0}}{|\mathbf{q}_x + \mathbf{G}'|^2} \delta(\omega - (\mathbf{G}+\mathbf{q}_x)\cdot\mathbf{v}_e)\,\delta(\omega - (\mathbf{G}'+\mathbf{q}_x)\cdot\mathbf{v}_e). \tag{4}$$

We assume an incident beam in the $z$-direction, which will produce scattered electrons with a range of momentum transfers in the $(x, y)$-plane perpendicular to the beam. Parallel to the beam the momentum transfer is fixed for a given energy-loss, $q_z = \omega/v_e$, so that for small losses in the order of few eV, we can assume $q_z = 0$. For the structure in question it is relevant to resolve the spectrum in terms of momentum transfers in the $x$-direction parallel to the ribbon, which can be done experimentally by moving the collection aperture away from the majority signal [1]. We get the final expression:

$$P(\omega, q_x) = \sum_{G_y, G'_y} \frac{e^{iG_y y_0}}{q_x^2 + G_y^2} \chi_{G_y,G'_y}(q_x,\omega) \frac{e^{-iG'_y y_0}}{q_x^2 + G'^2_y}, \tag{5}$$

given in terms of momentum transfer $q_x$, and where the sum over reciprocal lattice vectors is limited to the $y$-direction, taking $G_x, G_z = 0$. The position of the beam perpendicular to the wire, $y_0$, is varied in order to scan across the ribbon.

[1] E. Najafi, A. P. Hitchcock, D. Rossouw, and G. A. Botton, Ultramicroscopy **113**, 158 (2012).
